# Supplementary material for: Interfacial Effects on Solid Electrolyte Interphase in Lithium-ion Batteries
Source: arXiv:2010.16256 source file (2020-12-04)
Supplement: Supplementary file 1 [file suppinfo.pdf]

# Supporting Information: Interfacial Effects on Solid Electrolyte Interphase in Lithium-ion Batteries

Zeeshan Ahmad,[†] Victor Venturi,[†] Hasnain Hafiz,[†] and Venkatasubramanian Viswanathan[*,†,‡]

†*Department of Mechanical Engineering, Carnegie Mellon University, Pittsburgh, Pennsylvania 15213, USA*

‡*Department of Physics, Carnegie Mellon University, Pittsburgh, Pennsylvania 15213, USA*

E-mail: venkvis@cmu.edu

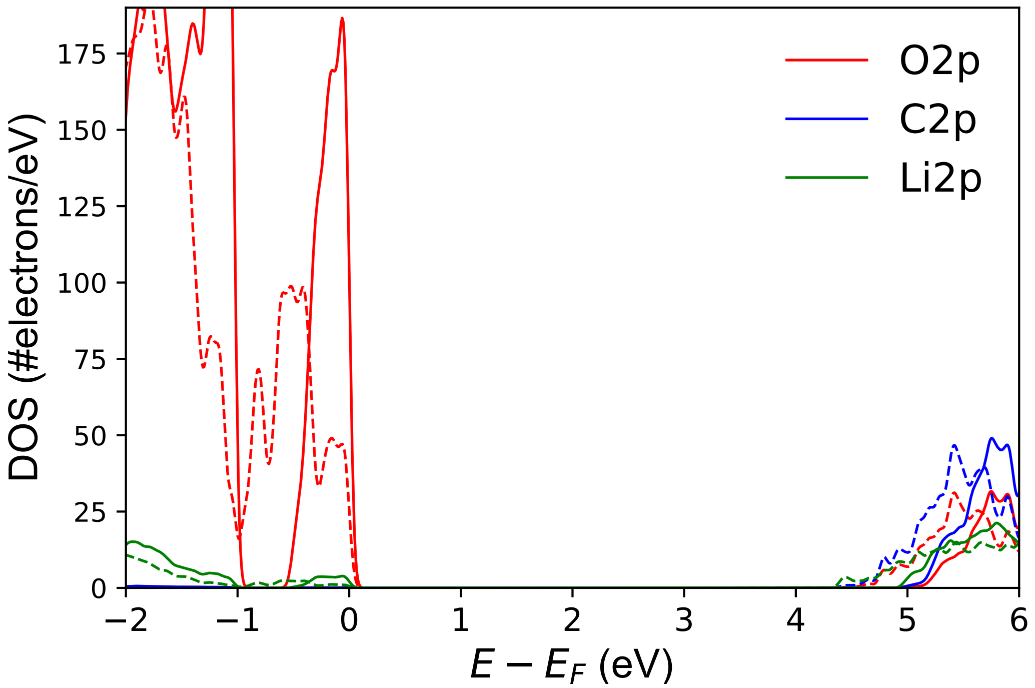


Figure S1: Comparison of electronic DOS of pristine and defective structures. The solid lines refer to pristine structure and the dashed lines refer to the defective structure. The Fermi level $E_F$ is set to VBM.

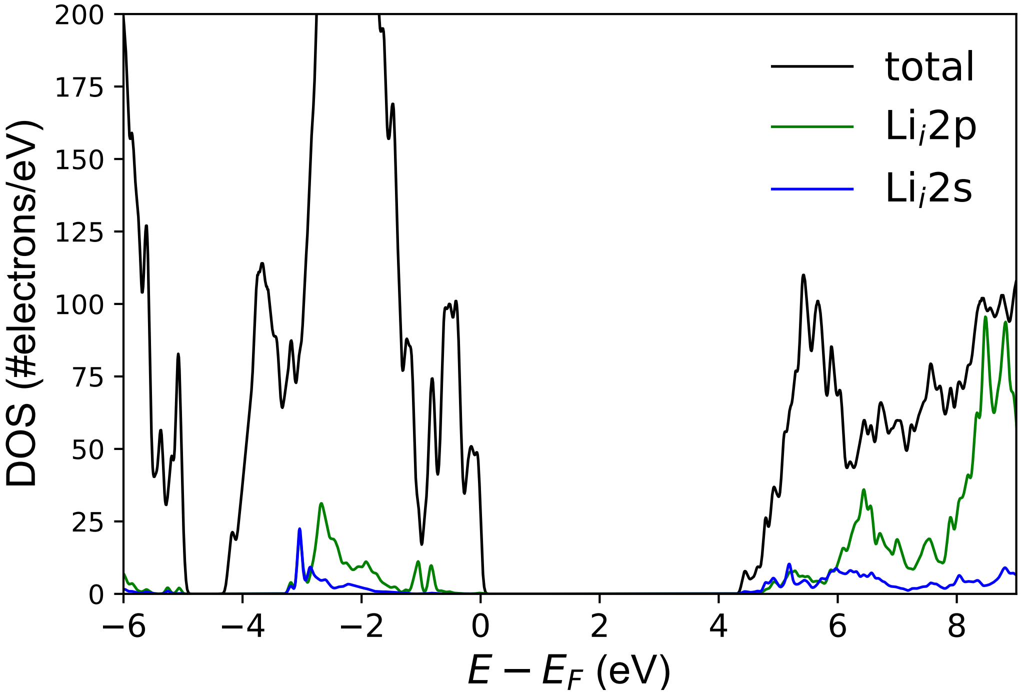


Figure S2: Electronic states of interstitial Li ($Li_i$) at the LiF-$Li_2CO_3$ interface. The Li interstitial DOS has been exaggerated by multiplying the no of states/eV with 100.

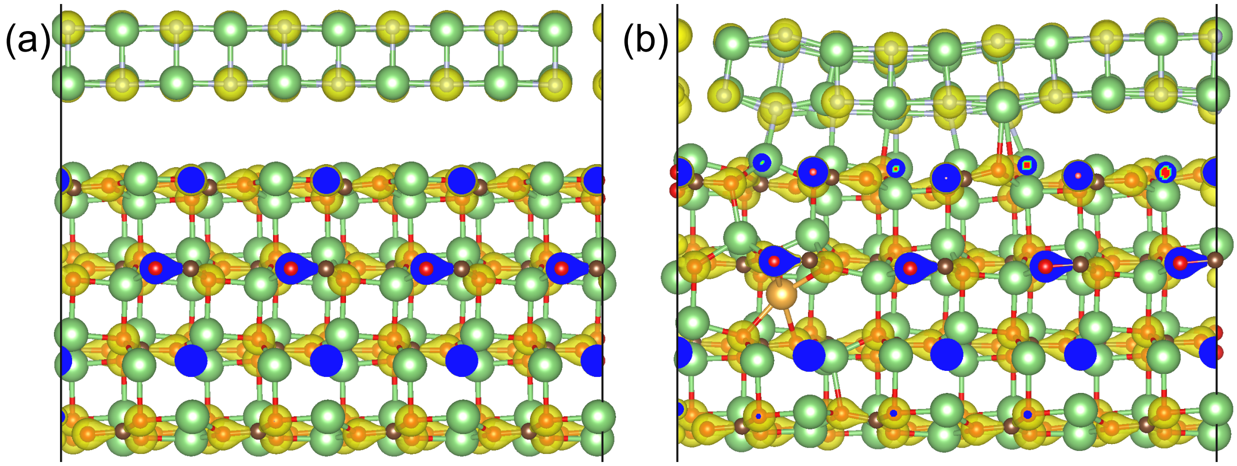


Figure S3: Electron density for the (a) pristine and (b) defective interfacial structure between LiF and $Li_2CO_3$. The Li interstitial defect in $Li_2CO_3$ is shown in yellow.

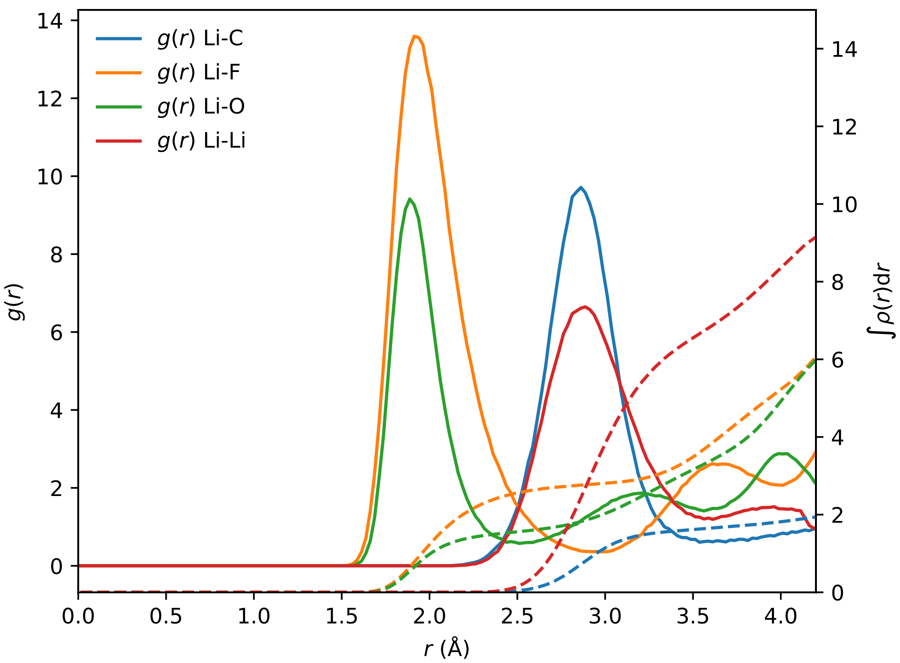


Figure S4: Radial distribution function $g(r)$ for the LiF-$Li_2CO_3$ interfacial structure at 600 K.

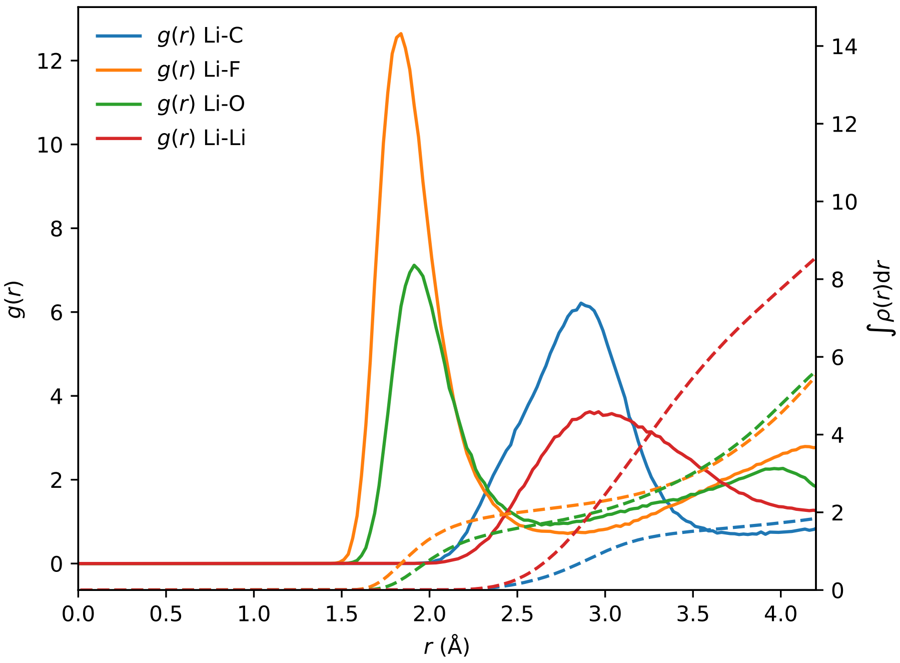


Figure S5: Radial distribution function $g(r)$ for the LiF-$Li_2CO_3$ interfacial structure at 800 K.

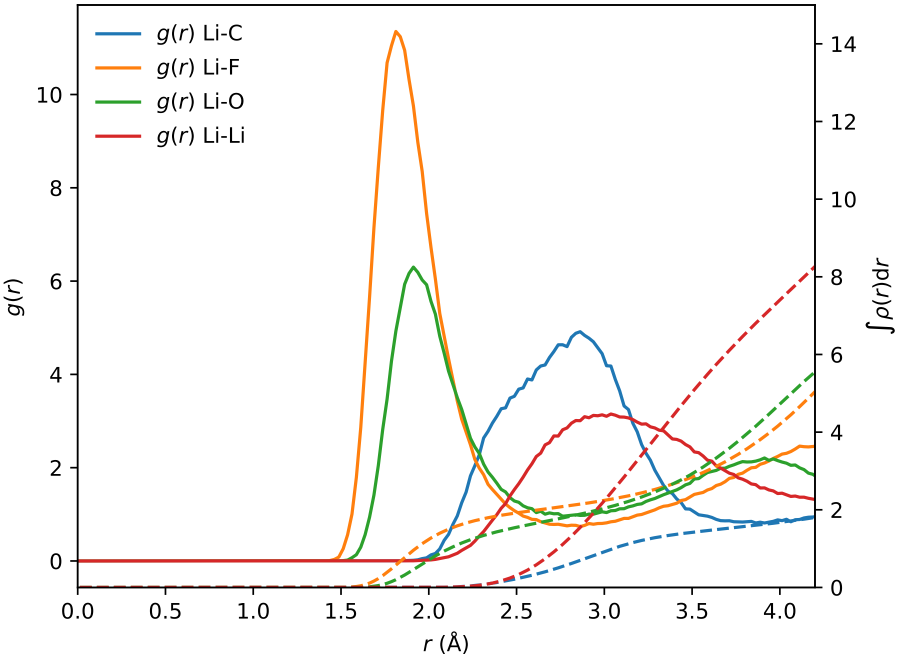


Figure S6: Radial distribution function $g(r)$ for the LiF-$Li_2CO_3$ interfacial structure at 900 K.

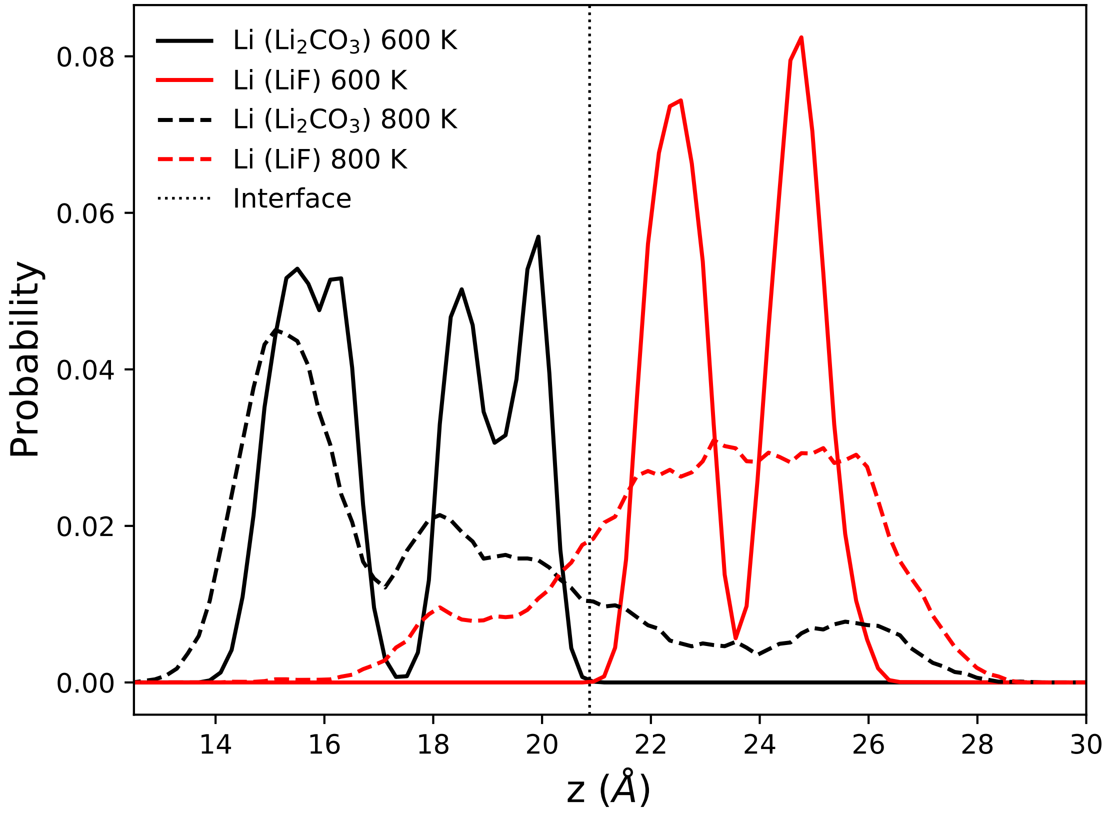


Figure S7: Probability density for the position of a Li ion as a function of the direction perpendicular to the interface $z$ at 600 and 800 K. The initial position of the interface, located near $z = 21$ Åis shown with a dotted line. The black and red lines represent Li initially in the $Li_2CO_3$ and LiF phases respectively. The plot demonstrates significant exchange of Li ions between LiF and $Li_2CO_3$ at 800 K which is not present at 600 K.
